# Supplementary material for: PGE: Robust Product Graph Embedding Learning for Error Detection
Source: arXiv:2202.09747 source file (2022-02-20)
Supplement: Supplementary file 1 [file appendix.tex]

\section{Appendix}
\appendix
\section{Experimental Details.}\label{sec_appendix_E}
\subsection{Inductive Setting.}
\begin{table*}
\centering
\resizebox{\linewidth}{!}{
 \begin{tabular}{cccc} 
  \toprule 
Head & Relation & Predicted Tail by TransE & Predicted Tail by PGE-RotatE\\ 
\midrule 
  \tabincell{c}{Nestle Coffee mate Coffee Creamer,\\ Hazelnut, Liquid Creamer Singles, \\Box of 50 Singles (Pack of 4) }& flavor & \tabincell{c}{watermelon/fruit punch/ \\ bacon/pumpkin/lavender} & \tabincell{c}{\textit{chocolate hazelnut}/salted caramel/ \\\textbf{hazelnut}/ Creamer} \\
 \midrule 
  \tabincell{c}{Ground Black Pepper (Black Pepper, Small)}& flavor & \tabincell{c}{unscented/vanilla mint/ \\ black cherry/organic/original} & \tabincell{c}{\textit{spicy}/garlic/cajun/ \\ \textit{pepper}/ \textbf{black pepper}}\\
  \midrule 
  \tabincell{c}{GNewman's Own Licorice Twists, Strawberry, \\ 5-Ounce Packages (Pack of 15)} & scent & \tabincell{c}{green-coffee-bean-extract-weight-loss-supplements/ \\ Amish Peanut Butter Spread, 9 oz/ \\ maple/habanero/ \\ Goya Black Beans 15.5oz - Frijoles Negros (Pack of 18)}  & \tabincell{c}{cucumber melon/ liquorice/ \\ cherry almond/ \textit{strawberries}/ \textbf{strawberry}}  \\
  \midrule 
  \tabincell{c}{Amish Peanut Butter Spread, 9 oz }& flavor & \tabincell{c}{mixed berry/strawberry lemonade/ \\ bulk wholesale supplies/ \\ blueberry/coconut fruit extract \\ cocos nucifera oil} & \tabincell{c}{\textit{peanut\-butter}/ \textit{peanut\_butter}/ \\ \textbf{peanut butter}} \\
\midrule 
  \tabincell{c}{Europa Essentials 100\% Pure Therapeutic \\ Grade Essential Oils, 36 Aromatherapy Scents \\ Collection – Patchouli, 10ml}& scent & \tabincell{c}{unsalted/neutral/citrus/ \\ hot chocolate/mocha}\ & \tabincell{c}{frankincense/ geranium/ \\ scent sandalwood/sandalwood/\textbf{patchouli}}  \\
  \bottomrule 
 \end{tabular} 
 }
 \caption{Case Study for inductive ability of PGE}
\label{case study for inductive setting.}
\end{table*}

\subsection{Case Study.}
\begin{table*}
\centering
\resizebox{\linewidth}{!}{
 \begin{tabular}{cccccc} 
  \toprule 
  \multicolumn{3}{c}{Identified Correct Triples} & \multicolumn{3}{c}{Missed Correct Triples} \\ 
Head & Relation & Tail & Head & Relation & Tail   \\ 
\midrule 
  \tabincell{c}{Muira Puama (Ptychopetalum Olacoides)\\  Tincture, Organic Liquid Extract \\ (Brand Name: HerbalTerra, \\ Proudly Made in USA) 30x2 fl.oz (30x60 ml)}& flavor & alcohol-based & \tabincell{c}{Bootleggers Coffee BBQ rub \\ - BARBECUE RUB - Beef, Chicken, Pork}& flavor & \textbf{original} \\
 \midrule 
  \tabincell{c}{Lenny \& Larry's The Complete Cookie, \\ Peanut Butter Chocolate Chip,  \\ 2 oz (Pack of 12) Soft Baked}& flavor & \tabincell{c}{peanut butter \\ chocolate chip}
 & \tabincell{c}{Baby Conditioner, Lavender Chamomile, \\ 16 Oz, 2 Pk}& scent & \textbf{conditioner} \\
  \midrule 
  \tabincell{c}{Deluxe Baby's Gift Basket \\ - Lavender Themed (Baby Oil and Soaps)}& scent & lavender & \tabincell{c}{The Bean Coffee Company Organic Unroasted \\ Green Coffee Beans, Colombian, 16-Ounce}& flavor & colombian \\
  \midrule 
  \tabincell{c}{Nature‚Äôs Blueprint Matcha Tea \\ - Organic Japanese UJI - Pure Ceremonial \\ Grade Green Tea Powder - 2 Pack Bundle \\ (2 oz.) - Whisk Up the Perfect Bowl, \\ or Gift to a Friend as a Set from Kyoto Japan.}& scent & green tea & \tabincell{c}{Stacy's Everything (Onion, Sesame, Poppy & Garlic) \\ Flavored Bagel Chips, 7 Ounce Bags (Pack of 12)}& flavor & everything \\
  \midrule 
  \tabincell{c}{Pharma-Grade, Pre-Separated Size 00 \\ Fillable Vegetarian Capsules 1000 Bulk \\ Pack in Resealable Bag. Flavorless Cellulose \\ Caps Snap Together Easily \& Hold Securely \\ for Custom Vitamins \& Nootropics}& scent & unscented
 & \tabincell{c}{Seventh Generation Chlorine Free Bleach, \\ Free & Clear, 64 oz
}& scent & \textbf{free} \\
  \bottomrule 
 \end{tabular} 
 }
 \caption{Identified correct triples v.s. missed correct triples. We present top 5 human labeled correct triples with highest score as examples of identified correct triples. Meanwhile, top 5 human labeled correct triples with lowest score are presented missed correct triples.}
 \label{case study of correct triple}
\end{table*}
